# Supplementary material for: Exposing and Mitigating Spurious Correlations for Cross-Modal Retrieval
Source: arXiv:2304.03391 source file (2023-04-06)
Supplement: Supplementary file 1 [file appendix.tex]

% % \begingroup
% % \let\clearpage\relax 
% % \onecolumn 

% % \begin{center}
% % \Large
% % Supplementary for \\
% % Exposing and Mitigating Spurious Correlations in Cross-Modal Retrieval
% % \end{center}



% % CVPR 2023 Paper Template
% % based on the CVPR template provided by Ming-Ming Cheng (https://github.com/MCG-NKU/CVPR_Template)
% % modified and extended by Stefan Roth (stefan.roth@NOSPAMtu-darmstadt.de)

% \documentclass[10pt,twocolumn,letterpaper]{article}

% %%%%%%%%% PAPER TYPE  - PLEASE UPDATE FOR FINAL VERSION
% % \usepackage[review]{cvpr}      % To produce the REVIEW version
% \usepackage{cvpr}              % To produce the CAMERA-READY version
% %\usepackage[pagenumbers]{cvpr} % To force page numbers, e.g. for an arXiv version

% % Include other packages here, before hyperref.
% \usepackage{graphicx}
% \usepackage{amsmath}
% \usepackage{amssymb}
% \usepackage{booktabs}
% \usepackage{xcolor}
% \definecolor{green}{rgb}{0.1, 0.5, 0.3}
% \usepackage{multirow}
% \usepackage{array}
% \usepackage{arydshln}
% \usepackage{float}

% % for pseudo-code
% \usepackage{listings}
% \definecolor{codegreen}{rgb}{0,0.6,0}
% \definecolor{codegray}{rgb}{0.5,0.5,0.5}
% \definecolor{codepurple}{rgb}{0.58,0,0.82}
% \definecolor{backcolour}{rgb}{0.95,0.95,0.92}
% \lstdefinestyle{mystyle}{
%     backgroundcolor=\color{backcolour},   
%     commentstyle=\color{codegreen},
%     keywordstyle=\color{magenta},
%     numberstyle=\tiny\color{codegray},
%     stringstyle=\color{codepurple},
%     basicstyle=\ttfamily\footnotesize,
%     breakatwhitespace=false,         
%     breaklines=true,                 
%     captionpos=b,                    
%     keepspaces=true,                 
%     numbers=left,                    
%     numbersep=5pt,                  
%     showspaces=false,                
%     showstringspaces=false,
%     showtabs=false,                  
%     tabsize=2
% }
% \lstset{style=mystyle, language=Python}



% \makeatletter
% \newcommand{\thickhline}{%
%     \noalign {\ifnum 0=`}\fi \hrule height 1.3pt
%     \futurelet \reserved@a \@xhline
% }
% \newcolumntype{"}{@{\hskip\tabcolsep\vrule width 1pt\hskip\tabcolsep}}
% \makeatother


% % It is strongly recommended to use hyperref, especially for the review version.
% % hyperref with option pagebackref eases the reviewers' job.
% % Please disable hyperref *only* if you encounter grave issues, e.g. with the
% % file validation for the camera-ready version.
% %
% % If you comment hyperref and then uncomment it, you should delete
% % ReviewTempalte.aux before re-running LaTeX.
% % (Or just hit 'q' on the first LaTeX run, let it finish, and you
% %  should be clear).
% \usepackage[pagebackref,breaklinks,colorlinks]{hyperref}


% % Support for easy cross-referencing
% \usepackage[capitalize]{cleveref}
% \crefname{section}{Sec.}{Secs.}
% \Crefname{section}{Section}{Sections}
% \Crefname{table}{Table}{Tables}
% \crefname{table}{Tab.}{Tabs.}

% %\newcommand{\metricAbbr}{DmAP@k\xspace}
% \newcommand{\metricAbbr}{ODmAP@k\xspace}
% \newcommand{\metricName}{object decorrelation\xspace}
% \input{math_commands.tex}
% \newcommand{\mypara}[1]{\vspace{2pt}\noindent{\bf{#1}}}
% %\newcommand{\myparagraph}[1]{\vspace{1pt}\noindent{\bf{#1}}}
% \newcommand{\todo}[1]{\textcolor{red}{TODO: #1}}
% \newcommand{\jm}[1]{\textcolor{cyan}{JM: #1}}
% \newcommand{\sophia}[1]{\textcolor{purple}{S: #1}}
% \newcommand{\zeynep}[1]{\textcolor{green}{Z: #1}}


% %%%%%%%%% PAPER ID  - PLEASE UPDATE
% \def\cvprPaperID{9} % *** Enter the CVPR Paper ID here
% \def\confName{CVPR Workshop (MULA)}
% \def\confYear{2023}


% \begin{document}

% %%%%%%%%% TITLE - PLEASE UPDATE
% \title{Supplementary for \\Exposing and Mitigating Spurious Correlations for Cross-Modal Retrieval}

% % \author{First Author\\
% % Institution1\\
% % Institution1 address\\
% % {\tt\small firstauthor@i1.org}
% % % For a paper whose authors are all at the same institution,
% % % omit the following lines up until the closing ``}''.
% % % Additional authors and addresses can be added with ``\and'',
% % % just like the second author.
% % % To save space, use either the email address or home page, not both
% % \and
% % Second Author\\
% % Institution2\\
% % First line of institution2 address\\
% % {\tt\small secondauthor@i2.org}
% % }
% \maketitle



% \section*{A. Matching table between noun phrases and class names.} 
% When synthesizing the text by removing noun phrase chunks, we should match the noun phrase with the class names of the object to be removed. While this (class name, noun phrase) pair is annotated in the Flickr30k dataset, we manually list the matching pair in the MS-COCO dataset. If the noun phrase contains a word related to the given class name, we regard that noun phrase as matching the given class name. The matching table is given in Table \ref{tbl:appendix:match}. These matching pairs are based on the implementation done in the  previous literature \cite{agarwal2020towards}, but we added and removed some pairs to make the pairs more relevant. For brevity, we did not list the word that is identical to the class name on the right-hand side of the table. 

% \section*{B. Analysis of distribution shift between the synthetic ($D’$) and the original ($D$) datasets.}
% % 
% \begin{table}[H]
% \centering\resizebox{0.3\textwidth}{!}{
% \vspace{-5pt}
% \begin{tabular}{lccc}
%         CLIP && ODmAP@1 & i2t R@1 \\
%         \cline{1-1}\cline{3-4}
%         \vspace{-1em} & \\
%         \cline{1-1}\cline{3-4}
%         \vspace{-1em} & \\
%         zero-shot && 58.6 & 50.6  \\
%         $D_s$ && 61.5 & 60.5 \\
%         $D'$ && 66.4 & 58.1  \\
%         $D\!\!+\!\!D'$ && 70.1 & 65.6  \\
%         \cline{1-1}\cline{3-4}
%     \end{tabular}
% }
% \vspace{-5pt}
% \end{table}
% As $|D’| < |D|$ (one-third smaller), we made a new dataset $D_s \subset D$ where $|D_s| = |D’|$ for comparison. Finetuning CLIP with $D’$ and $D_s$, respectively, resulted in pretty similar results (differing by 2.4\% i2t R@1). Considering the 9.9\% improvement from zero-shot to $D_s$, the data distribution of $D’$ seems not much shifted from the data distribution of $D$ even with somewhat broken visual and linguistic coherence in $D’$. 
% Also, compared to $D\!+\!D'$, $D'$ lowers ODmAP@1 by 3.7\%. We think this is because information on de-correlated objects in $D$ is not learned by the model trained only with $D'$.   

% \section*{C. Pseudo-code.} We present the pseudo-code for the implementation of our proposed data synthesis in Listing \ref{pseudocode:appendix}.


% %\clearpage
% {
% \setlength{\tabcolsep}{7pt}
% \renewcommand{\arraystretch}{1.2}
% \begin{table*}[t]
% \footnotesize
% \centering
% \begin{tabular}{ll}
% \hline
% \begin{tabular}[l]{@{}l@{}}Class name \\in MS-COCO\end{tabular} & Word in noun phrase chunk \\ \hline
% person & \begin{tabular}[l]{@{}l@{}} 
% man, woman, player, child, girl, boy, boys, people, lady, guy, kid, kids, surfer, cowboy, cowboys, \\
% adult, adults, cop, soldier, police, catcher, pitcher, jockey, baby, men, women, biker, spectator, rider, \\
% batter, gay, anyone, someone, reporter, somebody, anybody, everyone, worker, workers \end{tabular} \\
% airplane & plane, jet, aircraft \\
% bicycle & bike, biking, cycling \\
% motorcycle & motor \\
% bus & trolley \\
% car & van, taxi, trunk, truck, suv \\
% train & tram, subway \\
% traffic light & traffic \\
% stop sign & sign \\
% parking meter & meter \\
% fire hydrant & hydrant, hydrate, hydra \\
% bird & beak, duck, goose, gull, pigeon, chicken, penguin \\
% cat & kitty, kitten \\
% dog & puppy, puppies \\
% sheep & lamb \\
% horse & pony, foal \\
% cow & cattle, oxen, ox, herd, calves, bull, calf \\
% handbag & bag \\
% suitcase & bag, luggage, case \\
% frisbee & disc, disk, frisby \\
% sports ball & ball \\
% baseball bat & bat \\
% baseball glove & glove \\
% skateboard & board, skate \\
% surfboard & board \\
% snowboard & board \\
% skis & ski \\
% tennis racket & racket, racquet \\
% wine glass & glass, wine, beverage \\
% bottle & thermos, flask, beer, beverage \\
% cup & glass, mug, beverage, coffee, tea \\
% spoon & siverware \\
% donut & doughnut, dough \\
% cake & dessert, frosting \\
% dining table & desk, table, tables \\
% chair & stool \\
% potted plant & plant, flower \\
% vase & pot, vase \\
% tv & television, screen \\
% laptop & computer, monitor, screen \\
% cell phone & phone \\
% refrigerator & fridge \\
% book & novel \\
% scissors & scissor \\
% toothbrush & brush \\
% hair drier & drier \\
% teddy bear & teddy, toy, bear, doll \\
% \hline
% \end{tabular}
% % \vspace{-5pt}
% \caption{\textbf{Matching table between class names and noun phrases.} We regard the noun phrase as matching the given class name if the word related to the class name is contained in the noun phrase.}
% \vspace{-5pt}
% \label{tbl:appendix:match}
% \end{table*}
% }

% \clearpage
% \noindent\begin{minipage}{\textwidth}
% \begin{lstlisting}[language=Python, caption=Pseudo-code for the proposed data synthesis method to reduce spuriousness., label={pseudocode:appendix}]
% # Threshold for data synthesis (Section 3.1)
% alpha1 = 0.4
% alpha2 = 0.8
% alpha3 = 0.7

% # get synthetic data 
% for image_idx in ranger(n_images):
%     image, caption, bboxes, bbox_classnames = dataset.__getitem__(image_idx)
    
%     # extract nounphrases from caption using NLTK tool
%     nounphrases = get_nounphrases(caption)

%     # get masks for each classname in the image
%     classname_set = list(set(bbox_classnames))
%     mask_list = []
%     for classname_to_remove in classname_set:
%         bbox_idxs_to_remove = [i for i, _cat in enumerate(bbox_classnames) 
%                                if _cat == classname_to_remove]
%         bboxes_to_remove = bboxes[bbox_idxs_to_remove]
%         mask = union_bboxes(bboxes_to_remove) # union all the bboxes
%         mask_list.append(mask)

%     if len(classnames_set) >= 2:
%         for i, classname_to_remove in enumerate(classname_set):
%             # classname_to_remove to be removed
%             mask_q = mask_list[i]
%             mask_gs = [mask for j, mask in enumerate(mask_list) if j != i]
%             classname_gs = [_c for j, _c in enumerate(classname_set) if j != i]

%             # check size of removed region
%             if mask_q.sum() / (mask_q.size(2) * mask_q.size(3)) > alpha3:
%                 continue
                    
%             # check overlap between bbox from selected class and others
%             overlaps = torch.tensor(
%                 [torch.logical_and(mask_q, mask_g).sum() / mask_g.sum() 
%                  for mask_g in mask_gs])

%             # when removing a single class
%             if all(overlaps < alpha1):
%                 # synthetic image using inpainting GAN
%                 synth_image = synthesize_image(image, mask_q) 
%                 # synthetic caption using matching table in Appendix
%                 synth_caption = synthesize_caption(caption, classname_to_remove)
                
%             # when removing multiple classes
%             elif any(overlaps > alpha2):
%                 bool_overlaps = overlaps > alpha2
%                 mask_qs = \
%                     [mask_q] + [_m for j, _m in enumerate(mask_gs) if bool_overlaps[j]]
%                 classnames_to_remove = \
%                     [classname] + [_c for j, _c in enumerate(classname_gs) if bool_overlaps[j]]
%                 # synthetic image using inpainting GAN
%                 synth_image = synthesize_image(image, mask_qs)
%                 # synthetic caption using matching table in Appendix
%                 synth_caption = synthesize_caption(caption, classnames_to_remove)
% \end{lstlisting}
% \end{minipage}


% {\small
% \bibliographystyle{ieee_fullname}
% \bibliography{main}
% }

% % \endgroup

% \end{document}
